# Supplementary material for: Determining minimum energy conical intersections by enveloping the seam: exploring ground and excited state intersections in coupled cluster theory
Source: arXiv:2411.08207 source file (2024-11-14)
Supplement: Supplementary file 1 [file SI_tube.pdf]

**Supporting Information for “Determining  
minimum energy conical intersections by  
enveloping the seam: exploring ground and  
excited state intersections in coupled cluster  
theory”**

Sara Angelico, Eirik F. Kjørstad, and Henrik Koch\*

*Department of Chemistry, Norwegian University of Science and Technology, NTNU, 7491  
Trondheim, Norway*

E-mail: [henrik.koch@ntnu.no](mailto:henrik.koch@ntnu.no)

## Convergence of the algorithm: $S_1/S_2$ MECIs for uracil

To analyze the convergence of the algorithm, we study the  $S_1/S_2$   $\varepsilon$ -MECI in uracil using EOM-SCCSD. In Fig. 1 and 2, we compare the convergence properties of a stepwise optimization using the tube algorithm with the gradient projection method. All optimizations were converged to  $3 \cdot 10^{-4}$  au in the maximum element of the gradient and  $1.2 \cdot 10^{-4}$  au in the root mean square (rms) of the gradient. For the tube algorithm, we performed a first optimization with  $\varepsilon = 0.27$  eV and used the converged geometry as an initial guess for a second optimization with  $\varepsilon = 0.027$  eV.

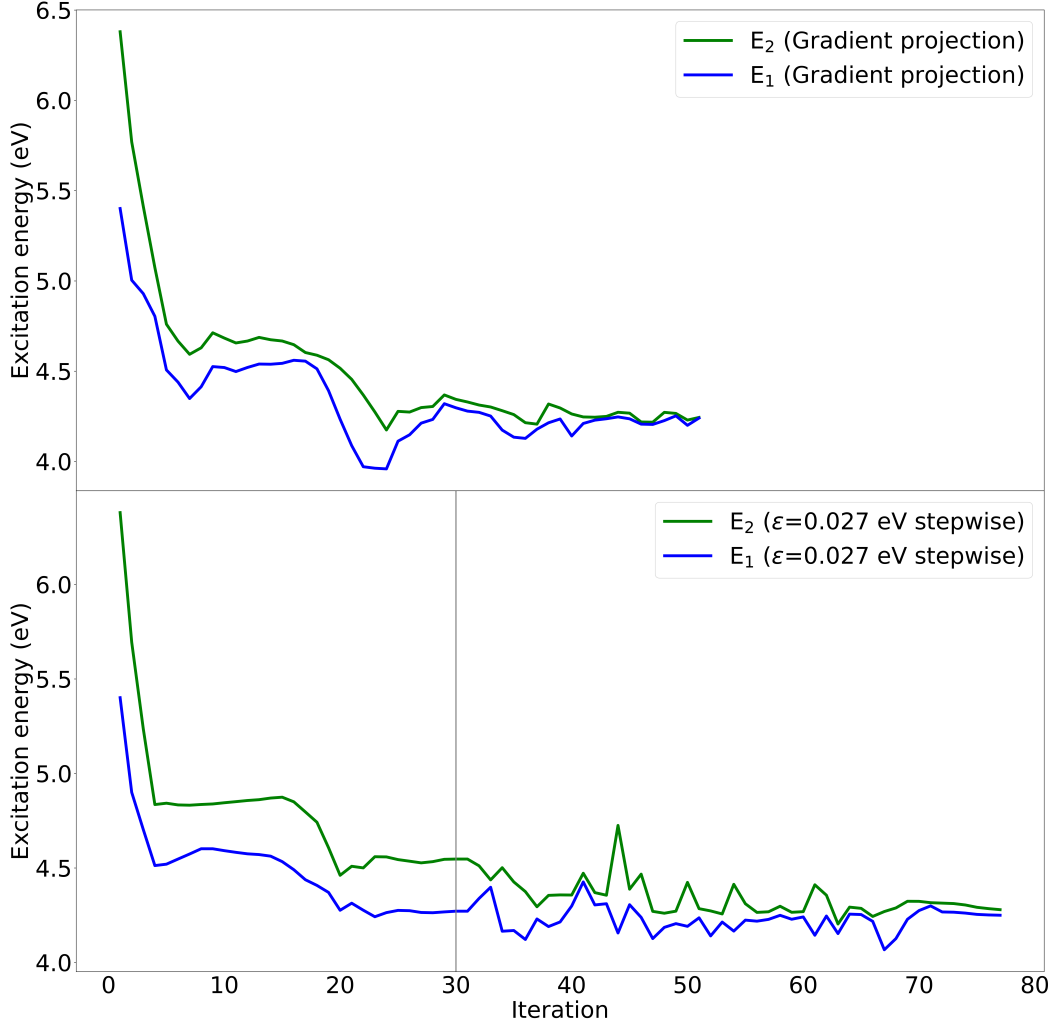

**Figure 1:** Excitation energies of  $S_1$  and  $S_2$  over the number of iterations for an optimization using the gradient projection method (top) and a stepwise optimization using the tube algorithm (bottom). The grey line indicates the first convergence of the stepwise tube algorithm with  $\varepsilon = 0.27$  eV.

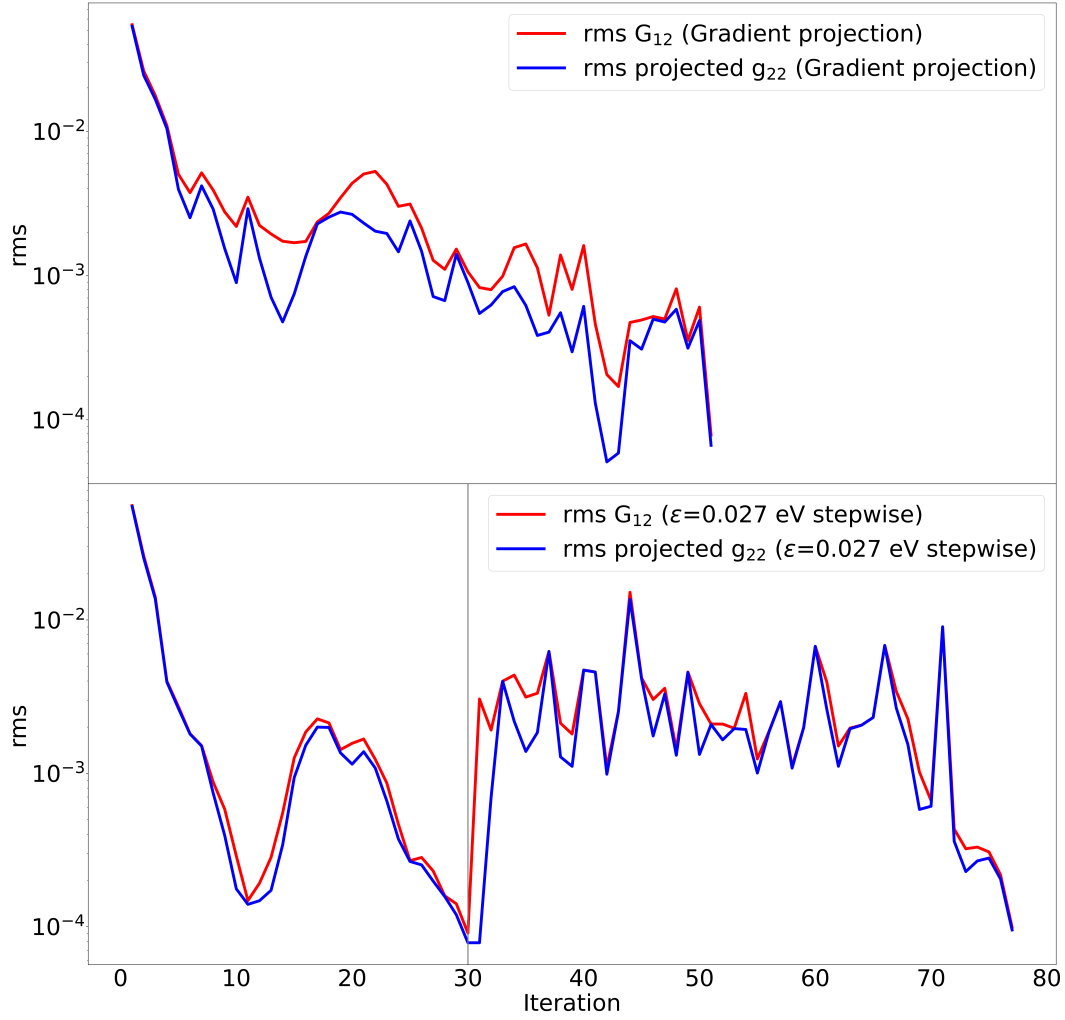

**Figure 2:** Root mean square displacement (rms) of the total gradient  $G_{12}$  and of the projection of  $g_{22}$  along the tube over the number of iterations for an optimization using the gradient projection method (top) and a stepwise optimization using the tube algorithm (bottom). The grey line indicates the first convergence of the stepwise tube algorithm with  $\epsilon = 0.27$  eV.

# Comparison of EOM-CCSD/EOM-SCCSD geometries for the $S_1/S_2$ MECIs for uracil ( $\varepsilon=0.027$ eV)

**Table 1:** Comparison of internal coordinates for the  $S_1/S_2$   $\varepsilon$ -MECI for uracil determined with  $\varepsilon = 0.027$  eV and using CCSD or SCCSD. Distances are given in angstrom ( $\text{\AA}$ ) and angles in degrees ( $^\circ$ ).  $E_1$  and  $E_2$  are excitation energies.

|       | C <sub>4</sub> -C <sub>5</sub> | C <sub>5</sub> -C <sub>6</sub> | $\angle N_1C_2N_3C_4$ | $\angle C_4C_5C_6N_1$ | $E_1$ (eV) | $E_2$ (eV) |
|-------|--------------------------------|--------------------------------|-----------------------|-----------------------|------------|------------|
| CCSD  | 1.41                           | 1.45                           | -30.5                 | -24.0                 | 4.245448   | 4.272669   |
| SCCSD | 1.41                           | 1.45                           | -30.5                 | -24.0                 | 4.245379   | 4.272599   |

## $S_0/S_1$ $\varepsilon$ -MECIs for uracil

In Table 2 we report the values of some relevant internal coordinates for the  $\varepsilon$ -MECIs for uracil varying the value of  $\varepsilon$ . For the *oop*-O geometry, the  $\varepsilon$ -MECI was converged up to  $\varepsilon=0.005$  Hartree. The  $^6S_5$   $\varepsilon$ -MECI was converged up to  $\varepsilon=0.0025$  Hartree. For energy differences lower than this values, we encountered convergence issues of the ground state CCSD equations.

**Table 2:** Comparison of internal coordinates for the uracil MECIs. Distances are given in angstrom ( $\text{\AA}$ ) and angles in degrees ( $^\circ$ ). CCSD  $\varepsilon$ -MECIs were converged with the cc-pVDZ basis set. Ref. 1: SF-TDDFT/6-31+G(d,p). Ref. 2: CASSCF(10/8)/6-31G\*.

| $\varepsilon$ (eV)             | CCSD |      |      | $^6S_5$               |                     | <i>oop</i> -O |      |      |                     |
|--------------------------------|------|------|------|-----------------------|---------------------|---------------|------|------|---------------------|
|                                | 0.27 | 0.14 | 0.07 | SF-TDDFT <sup>1</sup> | CASSCF <sup>2</sup> | 0.27          | 0.20 | 0.14 | CASSCF <sup>2</sup> |
| C <sub>4</sub> -O <sub>8</sub> | 1.21 | 1.21 | 1.21 | 1.20                  | 1.19                | 1.41          | 1.42 | 1.42 | 1.52                |
| C <sub>5</sub> -C <sub>6</sub> | 1.46 | 1.46 | 1.46 | 1.43                  | 1.45                | 1.35          | 1.35 | 1.35 | 1.34                |
| C <sub>4</sub> -C <sub>5</sub> | 1.49 | 1.49 | 1.49 | 1.47                  | 1.49                | 1.48          | 1.48 | 1.48 | 1.46                |
| $\angle C_4C_5C_6H_5$          | 113  | 114  | 114  | 121                   | 112                 | 179           | 179  | 179  | 179                 |
| $\angle C_6C_5C_4H_6$          | 21   | 22   | 22   | 24                    | 21                  | 1             | 1    | 1    | 1                   |
| $\angle C_4C_5C_6N_1$          | 50   | 51   | 52   | 53                    | 52                  | 1             | 1    | 0.5  | 1                   |
| $\angle C_2N_3C_4O_8$          | 163  | 165  | 166  | 161                   | -179                | 94            | 94   | 94   | 113                 |
| $\angle N_3C_4O_8$             | 119  | 119  | 119  | 119                   | 118                 | 85            | 85   | 85   | 82                  |

## S<sub>0</sub>/S<sub>1</sub> MECI for azobenzene

**Table 3:** Comparison of internal coordinates for the azobenzene CI-rot MECI (6-31G). 5SA-CASSCF(6/6) results are taken from Ref. 3. The  $\varepsilon$ -MECI for CCSD was converged with  $\varepsilon = 0.20$  eV. Distances are given in angstrom ( $\text{\AA}$ ) and angles in degrees ( $^\circ$ ).

|                        | N <sub>1</sub> -N <sub>2</sub> | C <sub>2</sub> -N <sub>1</sub> | N <sub>2</sub> -C <sub>3</sub> | $\angle$ C <sub>2</sub> N <sub>1</sub> N <sub>2</sub> C <sub>3</sub> | $\angle$ C <sub>1</sub> C <sub>2</sub> N <sub>1</sub> N <sub>2</sub> | $\angle$ N <sub>1</sub> N <sub>2</sub> C <sub>3</sub> C <sub>4</sub> | $\angle$ C <sub>2</sub> N <sub>1</sub> N <sub>2</sub> | $\angle$ N <sub>1</sub> N <sub>2</sub> C <sub>3</sub> |
|------------------------|--------------------------------|--------------------------------|--------------------------------|----------------------------------------------------------------------|----------------------------------------------------------------------|----------------------------------------------------------------------|-------------------------------------------------------|-------------------------------------------------------|
| SA-CASSCF <sup>3</sup> | 1.24                           | 1.41                           | 1.36                           | 97                                                                   | 180                                                                  | -15                                                                  | 122                                                   | 149                                                   |
| CCSD                   | 1.30                           | 1.43                           | 1.39                           | 99                                                                   | 175                                                                  | -13                                                                  | 119                                                   | 134                                                   |

## References

- (1) Zhang, X.; Herbert, J. M. Excited-State Deactivation Pathways in Uracil versus Hydrated Uracil: Solvatochromatic Shift in the  $1\text{ n } \pi^*$  State is the Key. *J. Phys. Chem. B* **2014**, *118*, 7806–7817.
- (2) Nachtigallová, D.; Aquino, A. J.; Szymczak, J. J.; Barbatti, M.; Hobza, P.; Lischka, H. Nonadiabatic dynamics of uracil: Population split among different decay mechanisms. *J. Phys. Chem. A* **2011**, *115*, 5247–5255.
- (3) Yu, L.; Xu, C.; Zhu, C. Probing the  $\pi\text{ } \pi^*$  photoisomerization mechanism of cis-azobenzene by multi-state ab initio on-the-fly trajectory dynamics simulation. *Phys. Chem. Chem. Phys.* **2015**, *17*, 17646–17660.
